# Supplementary material for: Deep Hiearchical Multi-Label Classification Applied to Chest X-Ray Abnormality Taxonomies
Source: arXiv:2009.05609 source file (2020-12-30)
Supplement: Supplementary file 1 [file appendix.tex]

Denoting the network's output logits as $\hat{y}_{(.)}$, the predicted unconditional probability of label $m$ can be written as:
\begin{align}
\hat{p}_m = \prod_{m'}\dfrac{1}{1+\exp(-y_{m'})},
\end{align}
where we use $m'$ to denote $m'\in A(m)$ for notational simplicity.

The \ac{HLUP} \ac{CE} loss is calculated as:
\begin{align}
	L_{HLUP} &= -z_m\log(\hat{p}_{m}) -(1-z_m)\log(1-\hat{p}_{m}) \mathrm{,} \\
	&= -z_m\log\left(\prod_{m'} \dfrac{1}{1+\exp(-y_{m'})}\right) -(1-z_m)\log \left(1-\left(\prod_{m'} \dfrac{1}{1+\exp(-y_{m'})}\right)\right) \mathrm{,}
\label{eqn:raw}
\end{align}
where $z_m$ is the ground truth label of $m$. 

We would like to break up the second term in \eqref{eqn:raw} to produce the following formulation:
\begin{align}
L_{HLUP} &=-z_m \log\left(\prod_{m'}\dfrac{1}{1+\exp(-y_{m'})}\right) -(1-z_m)\log\left(\prod_{m'}\left(1-\dfrac{1}{1+\exp(-y_{m'})}\right)\right) + \gamma \\
&= \sum_{m'} \left( -z_m \log\left(\dfrac{1}{1+\exp(-y_{m'})}\right) -(1-z_m)\log\left(1-\dfrac{1}{1+\exp(-y_{m'})}\right) \right)+ \gamma,
\label{eqn:better_raw}
\end{align}
which can be simplified to a sum of individual \ac{CE} losses plus $\gamma$:
\begin{align}
L_{HLUP} = \sum_{m'}\ell_{m'} +\gamma \textrm{,} \label{eqn:first}
\end{align}
where $\ell_{m}$ are individual cross entropy terms, using $z_m$ and $y_{m'}$ as the ground truth and logit input, respectively, and $\gamma$ is the scalar quantity we want to formulate. Note that \eqref{eqn:first} allows us to take advantage of numerically stable CE implementations, \eg{} those within Tensorflow, to calculate $\sum_{m'}\ell_{m'}$. 

To satisfy \eqref{eqn:better_raw}, we will need $\gamma$ to satisfy:
\begin{align}
-(1-z_m)\log\left(\prod_{m'}\left(1-\dfrac{1}{1+\exp(-y_{m'})}\right)\right) + \gamma &= -(1-z_m)\log \left(1-\left(\prod_{m'} \dfrac{1}{1+\exp(-y_{m'})}\right)\right), \nonumber \\
\log\left(\prod_{m'}\left(1-\dfrac{1}{1+\exp(-y_{m'})}\right)\right) - \frac{\gamma}{1-z_m} &= \log \left(1-\left(\prod_{m'} \dfrac{1}{1+\exp(-y_{m'})}\right)\right), \nonumber \\
\left(\prod_{m'}\left(1-\dfrac{1}{1+\exp(-y_{m'})}\right)\right) \exp(- \frac{\gamma}{1-z_m}) &= 1-\left(\prod_{m'} \dfrac{1}{1+\exp(-y_{m'})}\right).
\end{align}

Denoting 
\begin{align}
\alpha=\exp(- \frac{\gamma}{1-z_m}),
\label{eqn:alphasimple}
\end{align}
we have:
\begin{align}
	\alpha\left(\prod_{m'}\left(1-\dfrac{1}{1+\exp(-y_{m'})}\right)\right)&=1 - \prod_{m'}\dfrac{1}{1+\exp(-y_{m'})} \textrm{,} \label{eqn:alpha_pre} \\
    \alpha\left(\dfrac{\prod_{m' }\exp(-y_{m'})}{\prod_{m' }(1+\exp(-y_{m'}))}\right)&= \dfrac{\prod_{m'}(1+\exp(-y_{m'})) -1 }{\prod_{m'}(1+\exp(-y_{m'}))}\textrm{,} \\
    \alpha &=\dfrac{\prod_{m' }(1+\exp(-y_{m'})) -1}{\exp(\sum_{m'}-y_{m'})} \textrm{.}
    \label{eqn:alpha}
\end{align}
Substituting the left side of \eqref{eqn:alpha} into \eqref{eqn:alphasimple} gives us:
\begin{align}
    \gamma&=-(1-z_m)\log(\alpha) \nonumber \\
	&=-(1-z_m)\left(\sum_{m'}y_{m'}+\log\left(\prod_{m'}(1+\exp(-y_{m'})) -1\right)\right) \textrm{.}
    \label{eqn:gamma_pre}
\end{align}
If the log-product term of \eqref{eqn:gamma_pre} is expanded, with $1$ subtracted, it will result in
\begin{align}
	\gamma=-(1-z_m)\left(\sum_{m'}y_{m'}+\log\left( \sum_{S \in \mathcal{P}(A(m))\setminus\{\emptyset\}} \exp\left(\sum_{j\in S}-y_{j}\right)\right)\right) \textrm{,} \label{eqn:gamma_expanded}
\end{align}
where $S$ enumerates all possible subsets of the powerset of $A(m)$, excluding the empty set. For example if there were two logits, $y_{1}$ and $y_{2}$, the summation inside the log would be:
\begin{align}
	\exp(-y_{1}) + \exp(-y_{2}) + \exp(-y_{1}-y_{2}) \textrm{.}
\end{align}
The expression in \eqref{eqn:gamma_expanded} can be written as
\begin{align}
	\gamma=-(1-z_m)\left(\sum_{m'}y_{m'}+\mathit{LSE}\left(\left\{\sum_{j\in S}-y_j \quad \forall S \in \mathcal{P}(A(m))\setminus\{\emptyset\} \right \}\right)\right) \textrm{,} \label{eqn:final_gamma_app}
\end{align}
where $\mathit{LSE}$ is the LogSumExp function. Many numerical packages, including TensorFlow, provide numerically stable implementations of $\mathit{LSE}$, and its derivative. By substituting \eqref{eqn:final_gamma_app} into \eqref{eqn:better_raw}, a numerically stable version of the \ac{HLUP} \ac{CE} loss can be calculated. 

Should the cardinality of the powerset be too high, the LogSumExp expression can be approximated as a maximum function, which can be calculated using an $O(|A(m)|)$ scan of $y_{m'}$ values:
\begin{align}
	\gamma &\approx-(1-z_m)\left(\sum_{m'}y_{m'}+\max\left(\left\{\sum_{j\in S}-y_j \quad \forall S \in \mathcal{P}(A(m))\setminus\{\emptyset\} \right \}\right)\right) \textrm{,} \\
	&=\begin{cases}
	-(1-z_m)\left(\sum_{m'}y_{m'}+\sum_{j: y_{j}<0}{-y_{j}}\right) \textrm{,} & \text{if } \exists \, y_{m'} < 0 \\
	-(1-z_m)\left(\sum_{m'}y_{m'} +\max(\{-y_{m'}\})\right) \textrm{,} & \text{otherwise}
	\end{cases} \textrm{.}
\end{align}
